# Supplementary material for: Normal-state resistivity and the depairing current density of BaFe$_2$(As,P)$_2$ nanobridges along the $c$ axis
Source: arXiv:2408.09090 source file (2024-08-17)
Supplement: Supplementary file 1 [file supplementary_information_rev2.pdf]

# Supplemental Material for
# Normal-state resistivity and the depairing current density of $BaFe_2(As,P)_2$ nanobridges along the *c* axis

Yuki Mizukoshi[1], Kotaro Jimbo[1], Akiyoshi Park[2], Yue Sun[3], Tsuyoshi Tamegai[2], Haruhisa Kitano[1]

*[1]Department of Physics, Aoyama Gakuin University, Sagamihara 252-5258, Japan*

*[2]Department of Applied Physics, The University of Tokyo, Bunkyo-ku, Tokyo 113-8656, Japan*

*[3]Department of Physics, Southeast University, Nanjing 211189, China*

# I. Sample support

Figure S1 shows the details of sample support to perform the resistance measurements of a narrow bridge with a nanobridge along the *c* axis. This technique has also been used in the previous study on a small stack of the intrinsic Josephson junctions [1]. In this study, we used a closed cycle refrigerator system using two-stage GM refrigerator (Nikiglass and Sumitomo Industries) down to 4 K. Two heaters, which are located at the 2nd stage of the refrigerator and at the sample holder box, respectively, are mounted to control the temperature of the sample precisely. In order to avoid an accidental breakdown of the fabricated bridge, the sample was slowly cooled down with a rate of 15-20 K/h.

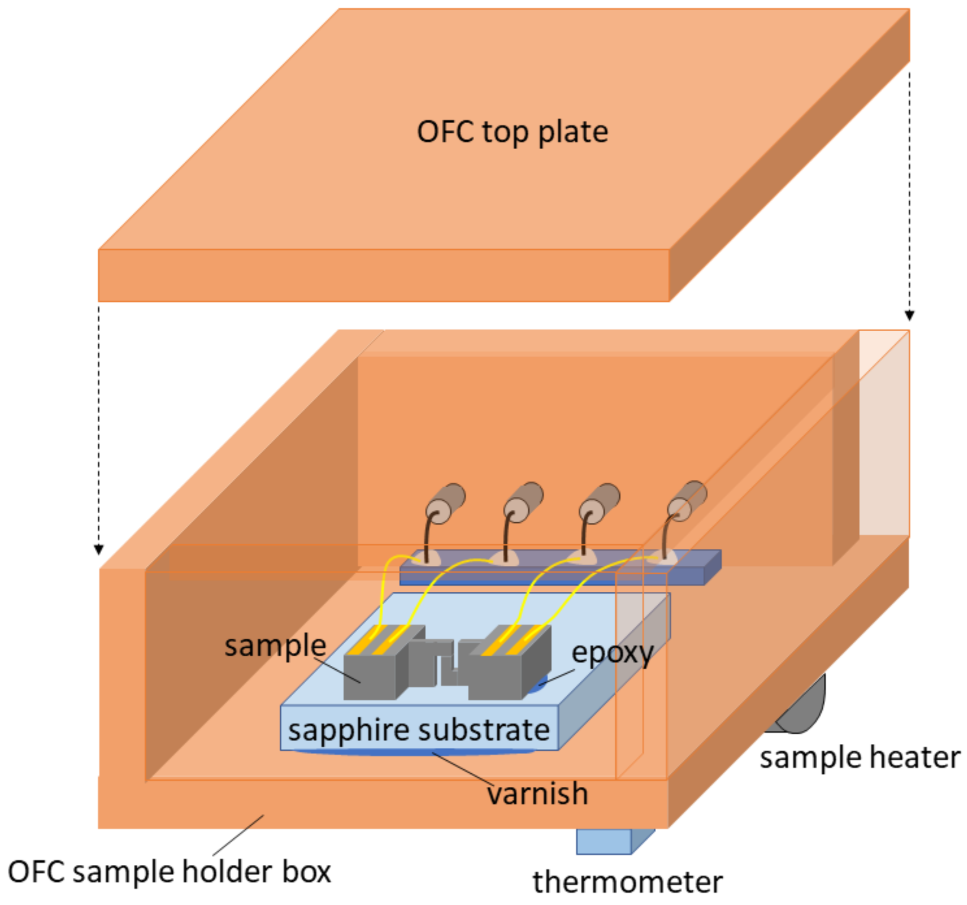


Fig. S1 Schematic viewgraph of sample support for resistance measurements.

## II. Geometrical effects in the FIB method to obtain the interlayer resistivity

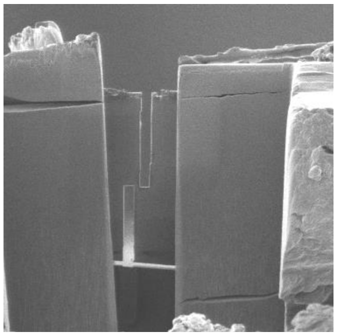

Fig. S2 Scanning ion microscopy (SIM) image of a narrow bridge with the c-axis nanobridge (bs05) and several cracks in the cleaved sample.

In the focused ion beam (FIB) fabrications, the etched surface is often damaged by FIB irradiation, causing the formation of an amorphous layer. The depth of such amorphous layers depends on materials as well as acceleration voltage and emission current of $Ga^+$ ions. In the previous transmission electron microscopy (TEM) study [2], we obtained the result that the thickness of FIB damage layer in $Bi_2Sr_2CaCu_2O_y$ cuprate superconductors was about 30 nm for the acceleration voltage of 30 kV (We used the same acceleration voltage in this study). On the other hand, we found that it is reduced to 5 nm in Fe(Te,Se) superconductors for the same acceleration voltage in a preliminary measurement. Thus, although we did not perform the TEM study for $BaFe_2(As,P)_2$ superconductors yet, we estimated that the thickness of FIB damage layer in this study was less than 30 nm. It is less than 15 % of the minimum size of the nanobridges fabricated in this study. In addition, we have rarely observed partial cracks in cleaved crystals when we made the $c$-axis nanobridges by the additional FIB fabrication. If small cracks were embedded into the cleaved samples, we can find them in a relatively simple way, by observing a sidewall of the narrow bridges in scanning ion microscopy (SIM) images. Figure S2 shows an example of such an observation of a partial crack in the cleaved sample, which is found to have a larger size than that of the $c$-axis nanobridge. Because of smallness in the fabricated nanobridge with dimensions less than 2 μm, a narrow bridge sample including a tiny crack inside is expected to be almost certainly broken down in the cooling process. Thus, we conclude that the obtained resistivity by the FIB method is not affected by the existence of partial cracks nor amorphous layers.

Rather, we consider that the uncertainty of the resistivity can be introduced by other factors. For instance, in the $R_1$ measurements to obtain $\rho_{ab}$, a narrow bridge with too small width should not be used. A slight slope of sidewall in the narrow bridge, which remains finite even after the FIB fabrication with a tilt angle of $\pm 1$ degree, makes the underestimation of bridge width, as shown in Fig. S3. Actually, we found that a width less than 1 μm led to the magnitude of $\rho_{ab}$ smaller than the values obtained by bulk measurements. We also found that the use of underestimated $\rho_{ab}$ in the analysis of $R_2$measurement overestimated the magnitude of $\rho_c$. Thus, we performed the $R_1$ measurement with an in-plane bridge (bp07) with a width of about 9 μm, before narrowing the bridge width to make the $c$-axis nanobridge.

Another point is the appropriate length of the $c$-axis nanobridges to obtain $\rho_c$ precisely. Although the elongation of a slit made in the sidewall of the bridge seems to increase the contribution of $R_c$ in the $R_2$ measurements, it actually increases both $R_{ab}$ and $R_c$, as shown in Fig. S4. Here, $\delta l$ is an increment of the length $l$ of nanobridge. In the $R_2$ measurement, the incremental resistance $\delta R$ due to $\delta l$ is given by a sum of $\rho_c \delta l / wh (= \delta R_c)$ and $\rho_{ab} l_L / \{w(t_L - \delta l)\} (= \delta R_{ab})$, where $w$ and $h$ are lateral sizes of the $c$-axis nanobridge. $l_L$ and $t_L$ are the length and thickness of the in-plane block on the elongated slit, respectively. When the ratio $\rho_c/\rho_{ab}$ is not so large, the divergent behavior of $\delta R_{ab}$ becomes more dominant than the linear increase of $\delta R_c$ with approaching $\delta l$ to $t_L$. We performed another set of $R_1$ and $R_2$ measurements using other two samples (bp20, bp21), in order to check the influence of the nanobridge length to the estimation of $\rho_c$. The $R_2$ measurement was done twice for each sample, where the length of the $c$-axis nanobridge was elongated by the additional FIB fabrication after the first $R_2$ measurement. As shown in Fig. S5, we found that the use of the $c$-axis nanobridge with a length longer than 2 μm underestimated the magnitude of $\rho_c$. Thus, we conclude that the $c$-axis nanobridge with the length less than 1 μm is more useful for the precise estimation of $\rho_c$

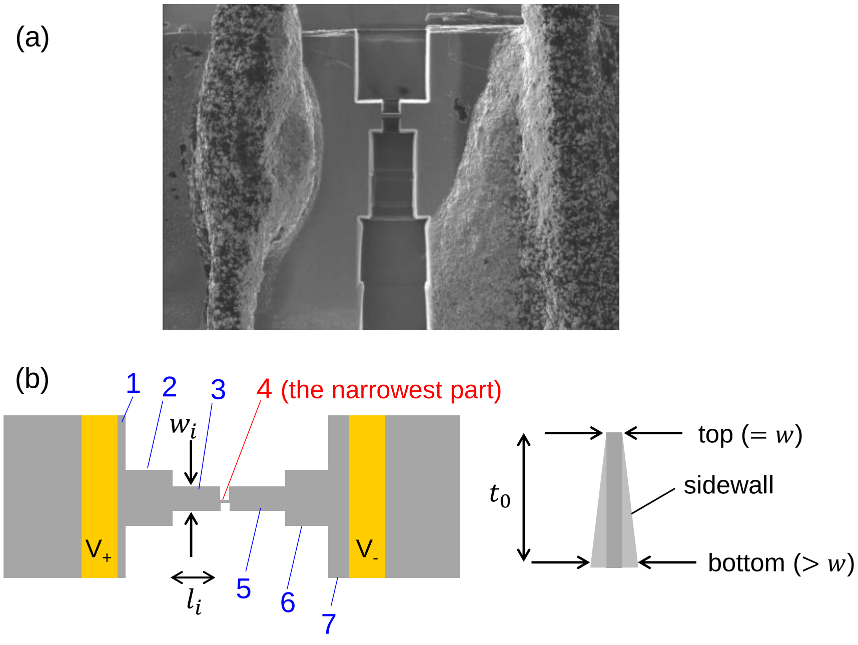


$$R_{\text{total}} = \frac{\rho_{ab}}{t_0} \times \sum \frac{l_i}{w_i} \Rightarrow \rho_{ab} = \frac{R_{\text{total}} t_0}{\sum (l_i / w_i)}$$

$$\sum \frac{l_i}{w_i} = \frac{l_1}{w_1} + \frac{l_2}{w_2} + \frac{l_3}{w_3} + \frac{l_4}{w_4} + \frac{l_5}{w_5} + \frac{l_6}{w_6} + \frac{l_7}{w_7}$$

Fig. S3 An example of the $R_1$measurement. (a) Top view of SIM image for a narrow bridge. (b) Schematic viewgraph to explain each size in the narrow bridge and a method to obtain $\rho_{ab}$.

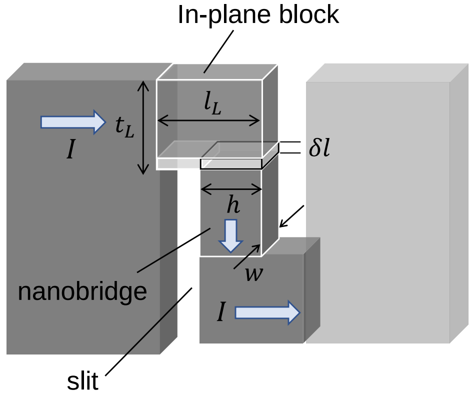


Fig. S4 Schematic viewgraph to explain the effect of an increment od the *c*-axis nanobridge length.

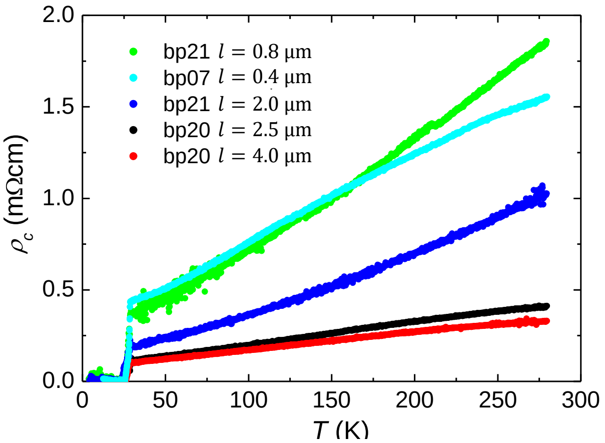


Fig. S5 Temperature dependence of $\rho_c(T)$, which was obtained from the $R_1$ and $R_2$ measurements.

in the $R_2$ measurements.

## III. EDX analyses for narrow bridges

We performed the energy-dispersive X-ray (EDX) analysis using a silicon drift detector (Bruker XFlash 6|30). In order to check a change of P dopant concentration after the FIB fabrication, the fabricated bridges as well as bulk crystals were analyzed. We used an acceleration voltage of 20 kV. As shown in Table S-I, the concentration of P for a bulk sample was determined by probing 10 spots on a cleaved surface. The results show that the average value of $x$ is 0.32.

On the other hand, for the fabricated bridges, 3 spots on a sidewall of narrow bridges were probed, as shown in Fig. S6. We used the same acceleration voltage as that for bulk samples, in order to keep quantitative performance rather than to increase a spatial resolution. Incident electron beam also remained perpendicular to the sidewall of bridges without any tilt angle, while the rotation angle of the sample stage was adjusted so as to enhance the signal to noise ratio, as shown in Fig. S7(a). This is because X-rays generated from the fabricated bridges with a hubbly sidewall and asymmetric property stemming from the existence of substrate is considered to have a sort of directionality. Actually, we found that the X-ray count rate was rapidly increased (above 100 kcps) when the bridge direction was parallel to an aperture plane of the

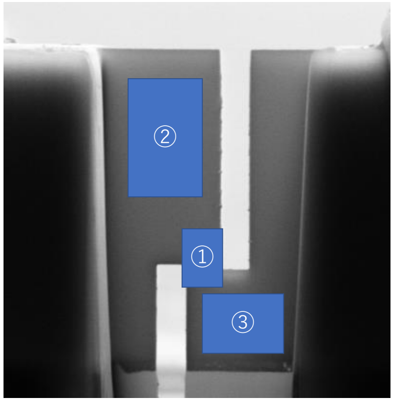


Fig. S6 Side view of SIM image of a narrow bridge with the c-axis nanobridge and 3 spots for EDX analysis.

detector and the substrate was farther than the bridge from the detector. Furthermore, in contrast to the EDX analyses of bulk crystals, we added gallium, silver, aluminum, carbon and oxygen to the candidates for elements detected in EDX analyses, since such elements were actually in the neighborhood of the bridges, as shown in Fig. S7(b). In order to upgrade the quantitative capability in EDX analyses, we made much account of data sets showing that total weight percentage was above 90 % in the analysis results for 3 positions in each sample. This means that the identification of the detected characteristic peaks of X-rays was almost complete. The results are shown in Table S-II.

We confirmed that most of the fabricated bridges except for bp07 and bp16 did not show unambiguous decrease of P dopant. On the other hand, the value of $x$ for bp16 was clearly decreased. This was also suggested by the two-staged superconducting transition observed in $R_2(T)$, as shown in Fig. S8. Here, it is considered that a lower $T_c$ corresponds to the value for the narrow bridge while a higher $T_c$ to that for the bulk part positioned between the voltage

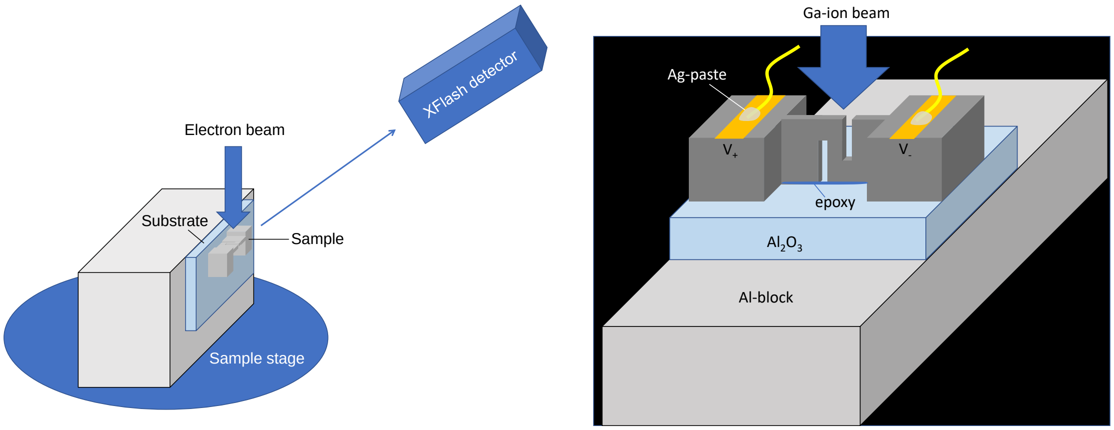


Fig. S7 (a) Schematic viewgraph of EDX analyses for the fabricated bridges.
(b) Schematic viewgraph of sample mount for EDX analyses.

terminals. Finally, it seems that the concentration of P dopant for bp07, used for the measurements of $\rho_c(T)$, is slightly decreased, in comparison to the results for bp06, bp18 and ij12. This observation is consistent with the fact that the temperature dependence of $R_2(T)$ for ij12, normalized by the value at 280 K shows a stronger linearity than that for bp07, as shown in Fig. S9. Thus, we conclude that although the FIB fabrication for P-doped Ba122 single crystals possibly makes a slight decrease of P dopant in the narrow bridge region, the decrement of P dopant concentration is less than 1%. We also confirmed that careful analyses of EDX spectra are quite useful for the determination of P concentration in the microfabricated region.

Table S-I Results of EDX analyses for a bulk sample.

| position | Ba | Fe | As | P | As+P | $x$ |
|---|---|---|---|---|---|---|
| 1 | 20.44 | 42.06 | 25.51 | 11.98 | 37.49 | 0.3196 |
| 2 | 20.24 | 41.72 | 25.88 | 12.16 | 38.04 | 0.3197 |
| 3 | 20.25 | 41.47 | 26.21 | 12.07 | 38.28 | 0.3153 |
| 4 | 20.99 | 41.41 | 26.08 | 11.52 | 37.60 | 0.3064 |
| 5 | 20.19 | 41.76 | 25.61 | 12.44 | 38.05 | 0.3269 |
| 6 | 20.27 | 42.04 | 25.65 | 12.04 | 37.69 | 0.3194 |
| 7 | 20.18 | 41.38 | 25.98 | 12.46 | 38.44 | 0.3241 |
| 8 | 20.12 | 41.72 | 25.92 | 12.25 | 38.17 | 0.3209 |
| 9 | 20.14 | 41.98 | 25.60 | 12.28 | 37.88 | 0.3242 |
| 10 | 20.13 | 41.85 | 25.87 | 12.14 | 38.01 | 0.3194 |
| average | 20.30 | 41.74 | 25.83 | 12.13 | 37.97 | 0.3196 |

Table S-II Results of EDX analyses for the fabricated bridges

| Sample | Spot No. | Ba (at.%) | Fe (at.%) | As (at.%) | P (at.%) | Ga (at.%) | Ag (at.%) |
|---|---|---|---|---|---|---|---|
| bp06 | 3 | 7.94 | 16.07 | 9.42 | 4.52 | 0.96 | 0.04 |
| bp07 | 2 | 5.82 | 7.29 | 3.97 | 1.84 | 0.34 | 0.26 |
| bp16 | 1 | 14.74 | 31.63 | 18.41 | 7.42 | 1.33 | 0.03 |
| bp18 | 1 | 14.17 | 27.74 | 14.15 | 6.66 | 1.52 | 0.20 |
| ij12 | 2 | 8.94 | 18.14 | 10.72 | 5.08 | 0.39 | — |
|  | 3 | 9.49 | 19.44 | 11.50 | 5.40 | 0.41 | — |

| Sample | Spot No. | Al (at.%) | C (at.%) | O (at.%) | $x$ | total (at.%) | total (wt.%) |
|---|---|---|---|---|---|---|---|
| bp06 | 3 | 2.42 | 51.12 | 7.51 | 0.324 | 100.00 | 99.87 |
| bp07 | 2 | 7.80 | 41.96 | 30.72 | 0.317 | 100.00 | 99.13 |
| bp16 | 1 | 26.44 | — | — | 0.287 | 100.00 | 100.77 |
| bp18 | 1 | 35.54 | — | — | 0.320 | 99.98 | 92.76 |
| ij12 | 2 | 10.35 | 27.10 | 19.28 | 0.322 | 100.00 | 93.86 |
|  | 3 | 10.62 | 24.64 | 18.50 | 0.320 | 100.00 | 93.08 |

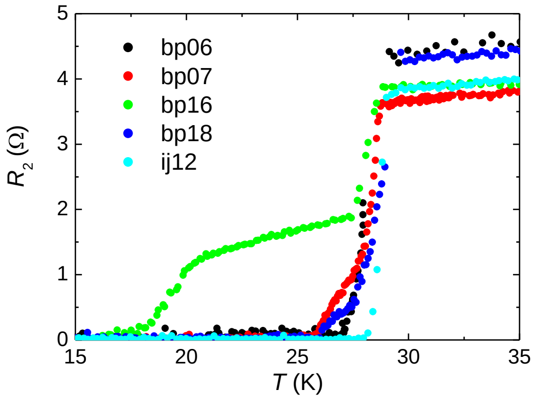


Fig. S8 Temperature dependence of $R_2(T)$ for the fabricated bridges.

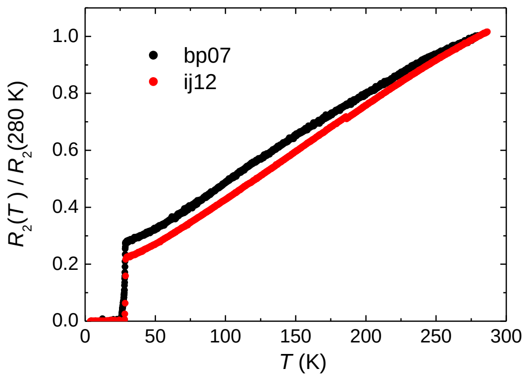


Fig. S9 Temperature dependence of $R_2(T)$ for bp07 and ij12, normalized by the value at $T = 280$ K.

**References:**


[1] K. Ota, K. Hamada, R. Takemura, M. Ohmaki, T. MacHi, K. Tanabe, M. Suzuki, A. Maeda, and H. Kitano, Comparative study of macroscopic quantum tunneling in $Bi_2Sr_2CaCu_2O_y$ intrinsic Josephson junctions with different device structures, Physical Review B - Condensed Matter and Materials Physics 79, 10.1103/PhysRevB.79.134505 (2009).

[2] Y. Kakizaki, J. Koyama, A. Yamaguchi, S. Umegai, S. Y. Ayukawa, and H. Kitano, Transmission electron microscopy study of focused ion beam damage in small intrinsic Josephson junctions of single crystalline $Bi_2Sr_2CaCu_2O_y$, Japanese Journal of Applied Physics 56, 10.7567/JJAP.56.043101 (2017).
